# Supplementary material for: RESTOR: Knowledge Recovery in Machine Unlearning
Source: arXiv:2411.00204 source file (2025-05-26)
Supplement: Supplementary file 1 [file task_vector.tex]

\section{Task Vector}
\label{appendix:task_vector}
\begin{figure}[t]
    \centering
    \includegraphics[width=0.6\textwidth]{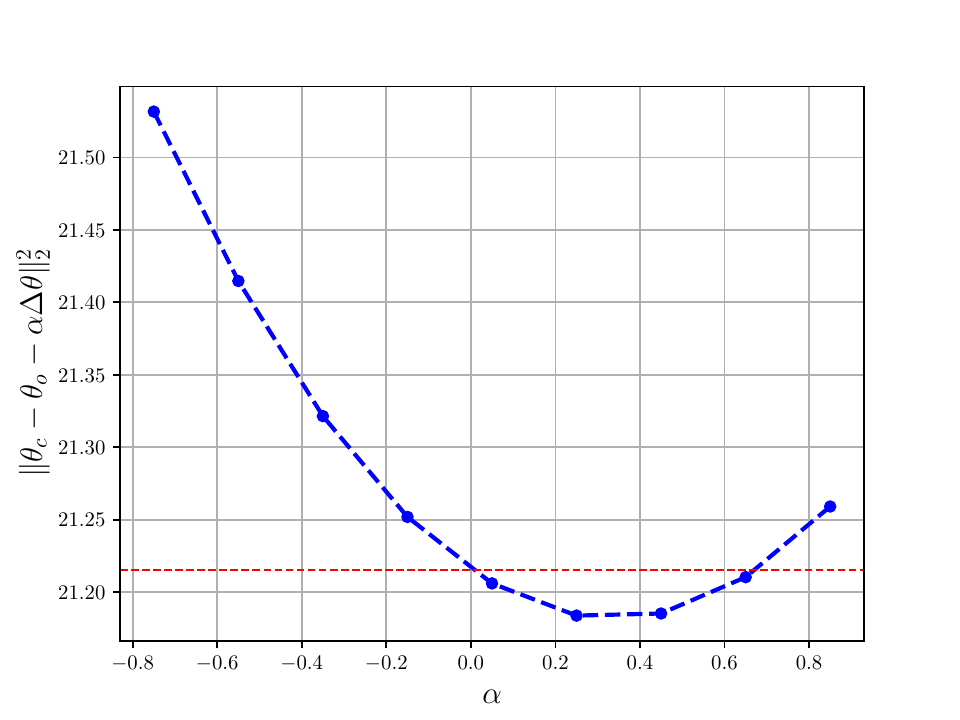}
    \caption{
    The value of $|\theta_c - \theta_0 - \alpha\Delta\theta|_2^2$ is evaluated across different $\alpha$ values. Red dotted lines indicate $|\theta_c - \theta_0|_2^2$. The direction obtained by the task vector $(\Delta \theta)$ does not align with $\theta_c - \theta_0$, indicating it cannot effectively guide the parameters back toward the clean state, $\theta_0$.
    Note that cosine similarity between $\theta_c - \theta_0$ and $\Delta \theta$ is $0.040$.
    }
    \label{fig:appendix:task_vector}
\end{figure}

In this section, we provide experimental details about task vector \citep{ilharco2022editing} when applied in our scenario.
task vector is implemented by obtaining a direction in parameter space, LoRA \citep{hu2021lora}, that corresponds to documents in the unlearning dataset.
This is done by continue fine-tuning the corrupted model for one more epoch.
Let $\theta_c$ be the corrupted model parameters and $\theta_*$ be the fine-tuned model parameters.
Task vector direction denoted by $\Delta\theta$ is then defined as $\Delta\theta = \theta_* - \theta_c$.
Then, the unlearned model parameters are \begin{align*}
    \theta_{\text{unlearned}} = \theta_c - \alpha\  \Delta \theta.
\end{align*}

To revert the model to its clean state,
$\Delta \theta$ should ideally be informative,
such that $\theta_c - \alpha \Delta \theta$ effectively undoes the corruption.
Specifically, if $\theta_0$ denotes the clean parameters,
then $\Delta \theta$ should align with $\theta_c - \theta_0$.
However, we find that in our case, this alignment does not occur,
as the model has overfitted to the corruption dataset. Figure~\ref{fig:appendix:task_vector} demonstrates that,
while the task vector direction does revert the corrupted model to some extent,
it is insufficient to restore the clean parameters fully.
Our evaluation of the task vector supports this analysis,
as it fails to enhance the corrupted model’s accuracy,
yielding results comparable to the corrupted models.
