# Supplementary material for: RESTOR: Knowledge Recovery in Machine Unlearning
Source: arXiv:2411.00204 source file (2025-05-26)
Supplement: Supplementary file 2 [file task_vector.tex]

\begin{figure}[t]
    \centering
    \includegraphics[width=0.6\textwidth]{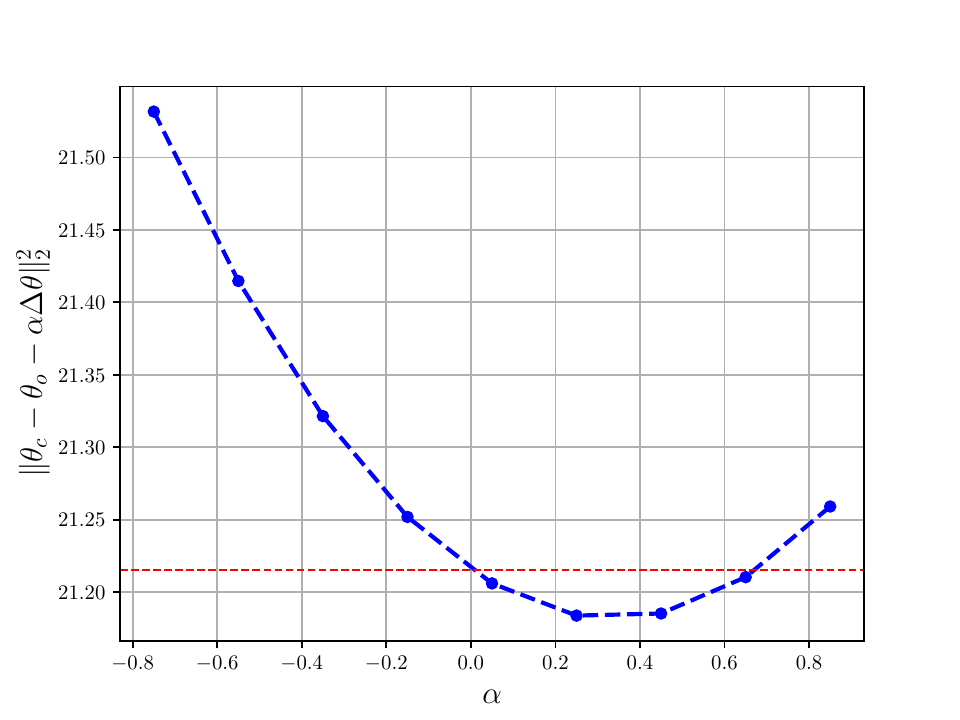}
    \caption{
    The value of $|\theta_c - \theta_0 - \alpha\Delta\theta|_2^2$ is evaluated across different $\alpha$ values. Red dotted lines indicate $|\theta_c - \theta_0|_2^2$. The direction obtained by the task vector $(\Delta \theta)$ does not align with $\theta_c - \theta_0$, indicating it cannot effectively guide the parameters back toward the clean state, $\theta_0$.
    Note that cosine similarity between $\theta_c - \theta_0$ and $\Delta \theta$ is $0.040$.
    }
    \label{fig:appendix:task_vector}
\end{figure}
